# Supplementary material for: Self-supervised GAN Detector
Source: arXiv:2111.06575 source file (2022-03-07)
Supplement: Supplementary file 1 [file gan_test_supple.tex]

\begin{table*}[]
\centering
\caption{\textbf{Zero-shot cross-model performance.} }
\scriptsize
\resizebox{1.00\linewidth}{!}{%
\begin{tabular}{lccccccccccccccc|cc}
\hline
\multicolumn{1}{c}{\multirow{2}{*}{Model}} & \multicolumn{1}{c}{\multirow{2}{*}{\begin{tabular}[c]{@{}c@{}}number of training class\\ (real/fake)\end{tabular}}} & \multicolumn{2}{c}{StyleGAN} & \multicolumn{2}{c}{StyleGAN2} & \multicolumn{2}{c}{BigGAN} & \multicolumn{2}{c}{CycleGAN} & \multicolumn{2}{c}{StarGAN} & \multicolumn{2}{c}{GauGAN}& \multicolumn{2}{c}{Deepfake} & \multicolumn{2}{|c}{Mean}\\ \cline{3-18} 
& & Acc. & A.P. & Acc. & A.P. & Acc. & A.P. & Acc. & A.P. & Acc. & A.P.& Acc. & A.P. & Acc. & A.P. & Acc. & A.P. \\ \hline

Wang\cite{adam} & (1,1) & 50.4 & 79.3 & 68.2 & 94.7 & 50.2 & 61.3 & 50 & 52.9 & 50 & 58.2 & 50.3 & 67.6 & 50.1 & 51.5 & 52.7  & 66.5 
 \\
Frank~\cite{frank} & (1,1) & 68.5 & 80.7 & 60.8 & 77.3 & 72.1 & 63 & 57.6 & 56.6 & 80.1 & 76.3 & 74 & 95.5 & 54.4 & 59.4 & 66.8  & 72.7 
\\
Durall~\cite{watch_cvpr20} & (1,1) & 64.1 & 58.6 & 69.3 & 62.9 & 55.4 & 52.9 & 69.6 & 62.8 & 95.4 & 91.5 & 57.5 & 54 & 53.6 & 52 & 66.4  & 62.1 
  \\
\hline
Wang\cite{adam} & (2,2) & 52.8 & 82.8 & 75.7 & 96.6 & 51.6 & 70.5 & 58.6 & 81.5 & 51.2 & 74.3 & 53.6 & 86.6 & 50.6 & 51.5 & 56.3  & 77.7 
  \\
Frank~\cite{frank} & (2,2) & 70.8 & 83.8 & 61.2 & 75.6 & 74.9 & 76.2 & 74.8 & 76.8 & 91.7 & 97.5 & 89.2 & 98.4 & 52.8 & 53 & 73.6  & 80.2 
  \\
Durall~\cite{watch_cvpr20} & (2,2) & 63.5 & 58.1 & 68.7 & 62.4 & 56.4 & 53.5 & 63.5 & 58.2 & 89.8 & 83.1 & 56.5 & 53.5 & 53.3 & 51.7 & 64.5  & 60.1 
  \\
\hline

Wang\cite{adam} & (4,4) & 63.8 & 91.4 & 76.4 & 97.5 & 52.9 & 73.3 & 72.7 & 88.6 & 63.8 & 90.8 & 63.9 & 92.2 & 51.7 & 62.3 & 63.6  & 85.2 
 \\
Frank~\cite{frank} & (4,4) & 72.2 & 82.1 & 64.2 & 80.1 & 68.9 & 82.4 & 53.7 & 66.2 & 89.1 & 99.2 & 65.3 & 90.3 & 51.1 & 49.6 & 66.4  & 78.6 
  \\
Durall~\cite{watch_cvpr20} & (4,4) & 63.9 & 58.4 & 69 & 62.7 & 58.5 & 54.7 & 69.6 & 63.1 & 99 & 98.1 & 57 & 53.8 & 50.4 & 50.1 & 66.8  & 63.0 
 \\
\hline
Wang\cite{adam} & (20,20) & 71.4 & 96.3 & 67.5 & 93.4 & 60.9 & 83.3 & 83.8 & 94.3 & 84.6 & 93.6 & 79.3 & 98.1 & 51.1 & 66.3 & 71.2  & \textbf{89.3} \\
Frank~\cite{frank} & (20,20) & 81.8 & 91.7 & 71.4 & 93.0 & 76.0 & 87.8 & 62.8 & 77.3 & 96.9 & 99.4 & 73.9 & 93.1 &  48.6 & 48.3 & 73.1 & 84.4 \\
Durall~\cite{watch_cvpr20} & (20,20) & 64.7 & 59.0 & 69.2 & 62.9 & 59.4 & 55.3 & 66.9 & 60.9 & 98.5 & 97.1 & 57.2 & 53.9 & 52.2 & 51.3 & 66.9 & 62.9 \\
\hline
Our & (1,0) & 71.5 & 79.1 & 70.0 & 79.3 & 77.3 & 90.0 & 87.5 & 86.3 & 99.8 & 100. & 70.9 & 96.9 & 69.2 & 74.0 & \textbf{78.0} & 86.5 
 \\
\hline
\end{tabular}
}
\label{tab:cross_gan_supple}
\end{table*}
